# Supplementary material for: Physics-constrained deep neural network method for estimating parameters in a redox flow battery
Source: arXiv:2106.11451 source file (2022-03-04)
Supplement: Supplementary file 1 [file sec-supplement.tex]

% Assumption

\begin{enumerate}
	\item Only consider the species: $\mathcal{S}$ = \{V(II), V(III), V(IV), V(V), \ce{H+}, \ce{H2O}\}.
	\item All chemicals are distributed uniformly in the solute and instantaneous mixing with negligible reaction in the electrolyte tanks.
	\item The applied charge/discharge current is constant.
	\item Incompressible fluid.
	\item Membrane is assumed to be fully saturated with no accumulation.
	\item Cell potential is composed of the reversible voltage, and the activation and ohmic losses.
	\item Consier temperature effects
\end{enumerate}

% 2020 Choi
\textit{For the VRFB cell shown in Fig. 1 (b), the governing equations and relevant physical parameters are summarized in Table 1. Further, the source terms in the transport and charge convection equations are listed in Table 2. Here, we assumed a quasi-steady state [19] for the model, and isothermal and isotropic properties for the membrane and electrode; further we assumed the electrolyte as a dilute solution with electro- neutrality, negligible electromigration in the transport equations, no side reactions and crossover through the membrane, and plug flow in the porous electrode [18]. }
 
% surface density
 Differences between bulk and surface concentrations
 Due to the mass transport resistance from the bulk solution to the surface of the porous carbon electrode, the concentrations of the vanadium species on the surface of the porous electrode (cis) are (4) often different from those (ci) in the bulk.
 
 Key reference:
 [1] S. B. Lee et al., “Open data, models, and codes for vanadium redox batch cell systems: A systems approach using zero-dimensional models,” J. Electrochem. Energy Convers. Storage, vol. 17, no. 1, 2019.

\subsubsection{High-fidelity correction}
% Describe how to enhance prediction capacity
In Section \ref{sec:pinn}, the parameter estimation method by PINN was introduced. With the optimized parameters learned from the measurment, the PINN model leads to enhanced voltage prediction $E_{\mathcal{M}}^{cell}$. 
Although the 0D model with enhanced calibrated model parameters by the PINN approach results in  as evident by the comparative study in \textcolor{blue}{Section XX} 

Nevertheless, although the lumped models has been enhanced by the PINN approach with enhanced calibrated parameters, it is not comprehensive enough to capture the whole charging-discharge behaviours due to the \textcolor{blue}{XXX} .... Therefore, we introduce an addtional neural network to correct the original PINN prediction, coined as high-fidelity correction. In contrast, we called the PINN prediction based on 0D model as the low-fidelity model.

The idea of the high-fidelity correction is we introduce an additional DNN function $y_H(\theta_H)$ to minimize the mismatch between the low-fidelity solution $E^{cell}_{\mathcal{M}}$ and the given experimental measurements $E^*$, that is, minimizing the following loss function:
\begin{equation}\label{eq:loss_correction}
\mathcal{L}_{H} (\theta_H)  = \frac{1}{N} \sum_{n=1}^{N}  [(E^{cell}_{\mathcal{M}}(\vec{z}_n) + y_H(\vec{z}_n))- E_H^*(\vec{z}_n)]^2
\end{equation}
where the notations $N$ and $\vec{z}$ were defined in Eq. (\ref{eq:loss_pinn2}). Note that here the measurements $E_H^*$ are associated with the subscript "$H$", denoting that the data are used for training the high-fidelity correction DNN $y_H(\theta_H)$. The data set in principle can be different from $E^*$ used in Eq. (\ref{eq:loss_pinn2}), but we use the same data set in this study.

As can be seen in Eq. (\ref{eq:loss_correction}), the PINN model $E^{cell}_{\mathcal{M}}$ is also involved in the computation. If one has trained the optimal weights $\hat{\vec{\theta}}$ based on Eq. (\ref{eq:loss_pinn2}), the PINN prediction $E^{cell}_{\mathcal{M}}(\vec{z}_n;\hat{\vec{\theta}})$ can be directly with the optimal weights. However, our numerical study shows that by simultaneously learn the weights $\vec{\theta}$ for $\vec{\mu}$ and $\theta_H$ for $y_H(\theta_H)$ can yiedl higher accuracy for the PINN model. Thus, we define a total loss function:
\begin{equation}\label{eq:loss_MPINN}
\mathcal{L}  = \mathcal{L}_{\mathcal{M}} + \mathcal{L}_{H} (\theta_H)  = \frac{1}{N} \sum_{n=1}^{N}  [(E^{cell}_{\mathcal{M}}(\vec{z}_n) + y_H(\vec{z}_n))- E_H^*(\vec{z}_n)]^2
\end{equation}

%with  weights $\vec{\theta} = \{\theta_1,...,\theta_m\}$ involved in the computation needs to be solved. 
One way to solve 

There are two approaches to 

high-fidelity 

and denotes the measurements for training 

$E^{cell}_{\mathcal{M}}$ are 

%\begin{equation}\label{eq:loss_correction}
%\mathcal{L}_{H} (\theta_H) = \frac{1}{N^{x}} \sum_{q=1}^{N^{x}} \frac{1}{N^t_q} \sum_{l=1}^{N^t_q} [E^{cell}_{\mathcal{M}}(t_l;\hat{\vec{\mu}}(\vec{x}_q)) - E^*(t_l,\vec{x}_q)]^2
%\end{equation}

\begin{equation}\label{eq:loss_correction}
\mathcal{L}  = \mathcal{L}_{\mathcal{M}} + \mathcal{L}_{H} (\theta_H)  = \frac{1}{N} \sum_{n=1}^{N}  [(E^{cell}_{\mathcal{M}}(\vec{z}_n) + y_H(\vec{z}_n))- E_H^*(\vec{z}_n)]^2
\end{equation}

where the notations $N$ and $\vec{z}_n$ are defined in Eq. (\ref{eq:loss_pinn2}), and $E^{cell}_{\mathcal{M}}$ are $E_H^*$ denotes the measurements for 
but it is physics-agnostic

\textcolor{blue}{...continue...}

\textit{The lumped models served chiefly as monitoring and control tools for the VRFB system but they were not comprehensive enough to be employed in the cell design and optimization. Several lumped dynamic VRFB models employed in the past were capable of predicting the dynamic changes of the cell voltage output as well as the active species concentration under different operating conditions [14,15]. }
Although 0D model provided efficient prediction with negligible cost, its predictive accuracy
